# Supplementary material for: Nonlinearity in stock networks
Source: arXiv:1804.10264 ancillary file (2018-06-26)
Supplement: Supplementary file 1 [file nonlinearity_in_stock_networks_supplement_arxiv.pdf]

# Supplementary material to ‘Nonlinearity in stock networks’

David Hartman[1] and Jaroslav Hlinka[1]

[1]Institute of Computer Science, Czech Academy of Sciences, Prague, Czech Republic

## 1 Introduction

This material contains additional results evaluating the effects of supposed nonlinearity in stock networks constructed for various sets of stocks and parametrizations. The results presented in the main body of the work are for stocks from the NYSE100 index and are produced using the Pearson correlation coefficient and mutual information estimated using a box-counting algorithm with marginal equiquantization, with preset parameter (number of bins) equal to 4. We present our findings for the intervals 11 November 2003 – 7 November 2013 and 11 November 2003 – 11 November 2008. Moreover, all commonly used filterings are shown – namely MST, PMFG and WTA. In this supplement, we present similar findings for other stocks indices, namely the FTSE100 index, characterizing stocks at the London Stock Exchange, in Section 3, and the SP500 index of American stocks in Section 4. Additionally, in Section 2.1 we also present results of our analysis for the NYSE100 index when using the same estimator but with 8 bins instead of 4. For all three indices, we also give the results of our analysis restricted to those stocks traded for the whole duration of the interval under consideration; these are specified at the beginning of Section 2 for NYSE100, the beginning of Section 3 for FTSE100, and the beginning of Section 4 for SP500.

## 2 NYSE100 index

The original analysis is performed on set of stocks from NYSE100 index. The list of corresponding stocks is shown in Table 1. Since we are interested only in stocks traded between 11 November 2003 and 7 November 2013 we filter out these not present on the whole period, see Figure 1 showing the corresponding filtering.

Table 1: Table of considered companies as part of stocks index NYSE100 that were traded between 11 November 2003 and 7 November 2013.

| | | | |
|---|---|---|---|
| MMM | 3M Co | JPM | JPMorgan Chase & Co |
| ABT | Abbott Laboratories | KMB | Kimberly-Clark Corp |
| ACN | Accenture PLC | LMT | Lockheed Martin Corp |
| AGN | Allergan Inc. | LOW | Lowe's Cos Inc |
| MO | Altria Group Inc | MCD | McDonald's Corp |
| AXP | American Express Co | MDT | Medtronic PLC |
| AIG | American International Group Inc | MRK | Merck & Co Inc |
| APC | Anadarko Petroleum Corp | MET | MetLife Inc |
| APA | Apache Corp | MON | Monsanto Co |
| T | AT&T Inc | MS | Morgan Stanley |
| BAC | Bank of America Corp | NOV | National Oilwell Varco Inc |
| BAX | Baxter International Inc | NEM | Newmont Mining Corp |
| BMY | Bristol-Myers Squibb Co | NKE | NIKE Inc |
| CAT | Caterpillar Inc | OXY | Occidental Petroleum Corp |
| CVX | Chevron Corp | PEP | PepsiCo Inc |
| C | Citigroup Inc | PFE | Pfizer Inc |
| CL | Colgate-Palmolive Co | PX | Praxair Inc |
| COP | ConocoPhillips | PG | Procter & Gamble Co/The |
| GLW | Corning Inc | PRU | Prudential Financial Inc |
| CVS | CVS Health Corp | SLB | Schlumberger Ltd |
| DHR | Danaher Corp | SPG | Simon Property Group Inc |
| DE | Deere & Co | SO | Southern Co/The |
| DVN | Devon Energy Corp | SCCO | Southern Copper Corp |
| D | Dominion Resources Inc/VA | TGT | Target Corp |
| DUK | Duke Energy Corp | BK | Bank of New York Mellon Corp/The |
| DD | EI du Pont de Nemours & Co | BA | Boeing Co/The |
| LLY | Eli Lilly & Co | KO | Coca-Cola Co/The |
| EMR | Emerson Electric Co | DOW | Dow Chemical Co/The |
| EOG | EOG Resources Inc | GS | Goldman Sachs Group Inc/The |
| EXC | Exelon Corp | HD | Home Depot Inc/The |
| XOM | Exxon Mobil Corp | PNC | PNC Financial Services Group Inc/The |
| FDX | FedEx Corp | TRV | Travelers Cos Inc/The |
| F | Ford Motor Co | DIS | Walt Disney Co/The |
| BEN | Franklin Resources Inc | TWX | Time Warner Inc |
| FCX | Freeport-McMoRan Inc | USB | US Bancorp/MN |
| GD | General Dynamics Corp | UNP | Union Pacific Corp |
| GE | General Electric Co | UPS | United Parcel Service Inc |
| GIS | General Mills Inc | UTX | United Technologies Corp |
| HAL | Halliburton Co | UNH | UnitedHealth Group Inc |
| HON | Honeywell International Inc | VZ | Verizon Communications Inc |
| HPQ | Hewlett-Packard Co | WMT | Wal-Mart Stores Inc |
| ITW | Illinois Tool Works Inc | WBA | Walgreens Boots Alliance Inc |
| IBM | International Business Machines Corp | WFC | Wells Fargo & Co |
| JNJ | Johnson & Johnson | YUM | Yum! Brands Inc |

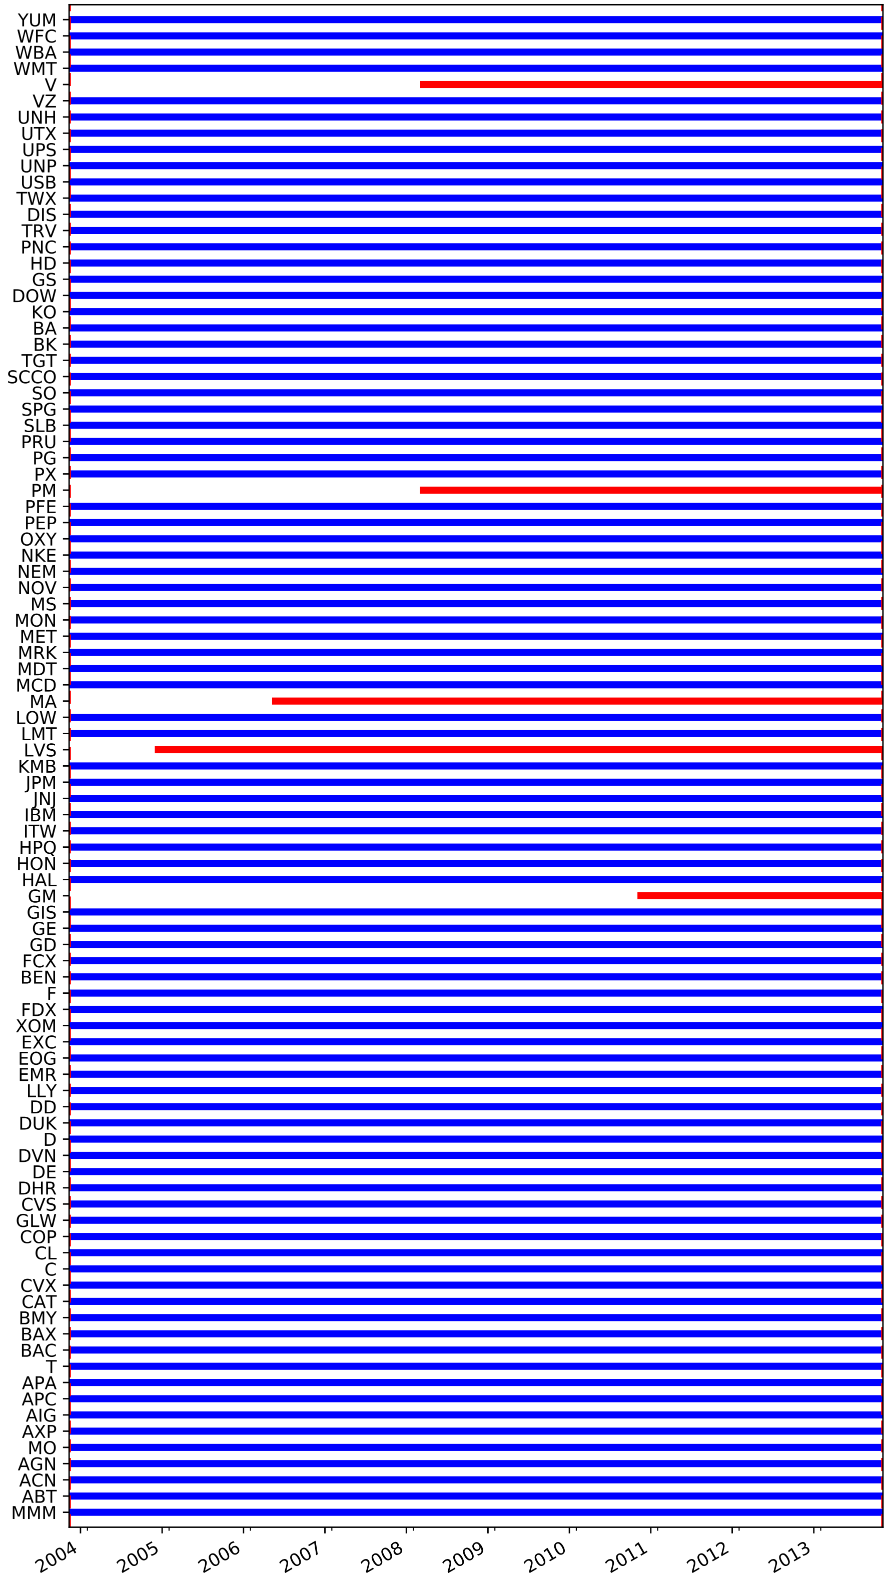


Figure 1: Plot showing existence intervals for stocks from NYSE100 index. Those traded between 11 November 2003 and 7 November 2013 are indicated blue, while others with shorter interval of existence are denoted as red.

## 2.1 Analysis of nonlinearity using MI estimator with 8 bins

This section contains results of the analysis using 8 bins for mutual information estimator. Relation between values of correlation coefficient and mutual informations are shown in Figure 2.

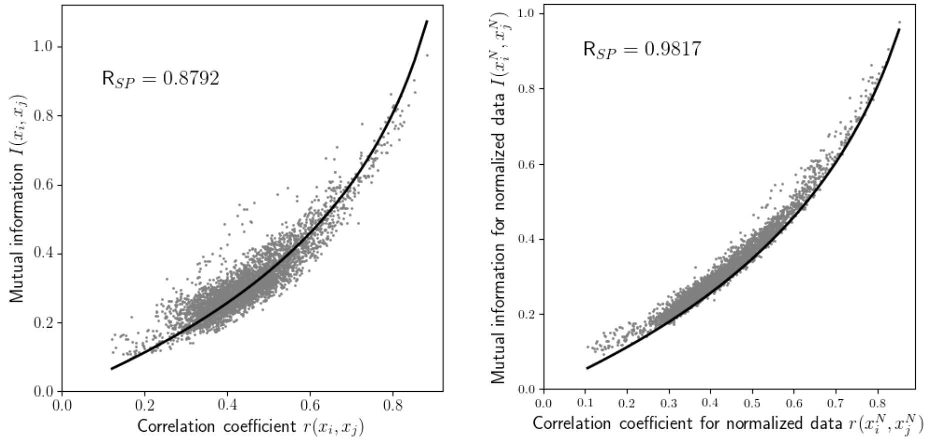


Figure 2: Relation between correlation and mutual information estimates from the original data (left) and marginally normalized data (right). Original data were log-returns of the close prices of the NYSE100 stocks. To estimate mutual information 8 bins are used for discretization. Each gray point represents the values of $r(x_i, x_j)$ and $I(x_i, x_j)$ (left) or $r(x_i^N, x_j^N)$ and $I(x_i^N, x_j^N)$ (right) for a pair of variables $x_i, x_j$ (left) or $x_i^N, x_j^N$ (right) for $i, j \in \{1, \ldots, N\}$. Gaussian mutual information $I_G$ shown by black line.

Localization of the remaining nonlinearity after normalization is presented in Figure 3 providing detection of a stock with the highest contribution and its further visualization.

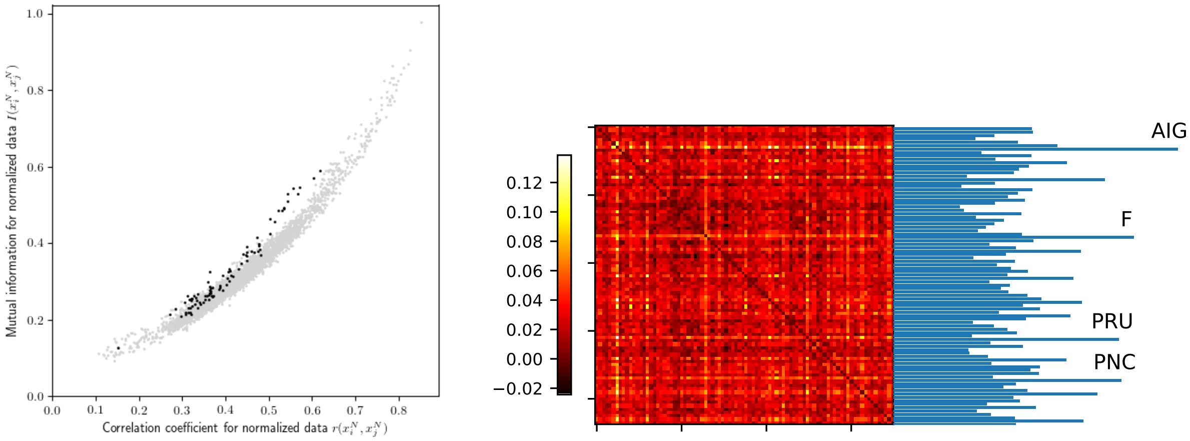


Figure 3: *Left*: Relation between correlation and mutual information estimates from the normalized data having similar setting as in Figure 2 with stock AIG highlighted in black. *Right*: Extranormal information $I_e$ for normalized data with summed rows and highlighted extremes.

With stock AIG removed further comparison of linear and nonlinear contribution can be done at the level of global network characteristics. Results are shown in Figure 4.

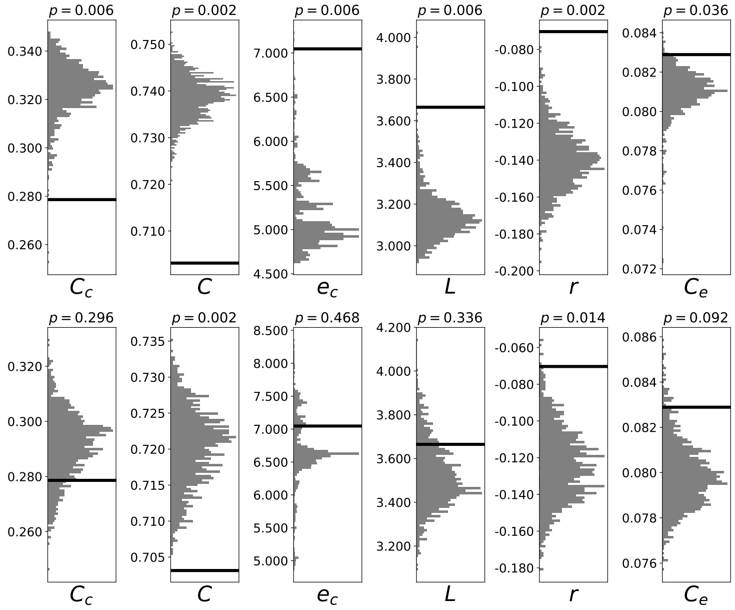


(a) Network from original data filtered using PMFG

(b) Network from marginally normalized data filtered using PMFG

Figure 4: Global graph characteristics computed for networks constructed from real data (blue bullets) and out of linearized surrogate datasets (gray bullets) both based on the NYSE100 index with the stock AIG removed. Connectivity has been computed using mutual information for original and marginally normalized data augmented with 99 linear surrogates. Presented characteristics are closeness $C_c$, average clustering coefficient $C$, eccentricity $e_C$, average shortest path $L$, assortative coefficient $r$ and eigenvalue centrality $C_e$.

There remain some contributions when resolving nonlinearity within PMFG. Considering results shown in Figure 4 it is not that strong as results of original analysis using estimator with 4 bins. In this case it is necessary to explore possible sources in more detail. Instead of analyzing extranormal information for all pairs as in Figure 3 we filter out only pairs responsible for PMFG network construction and analyze their contribution, see Figure 5.

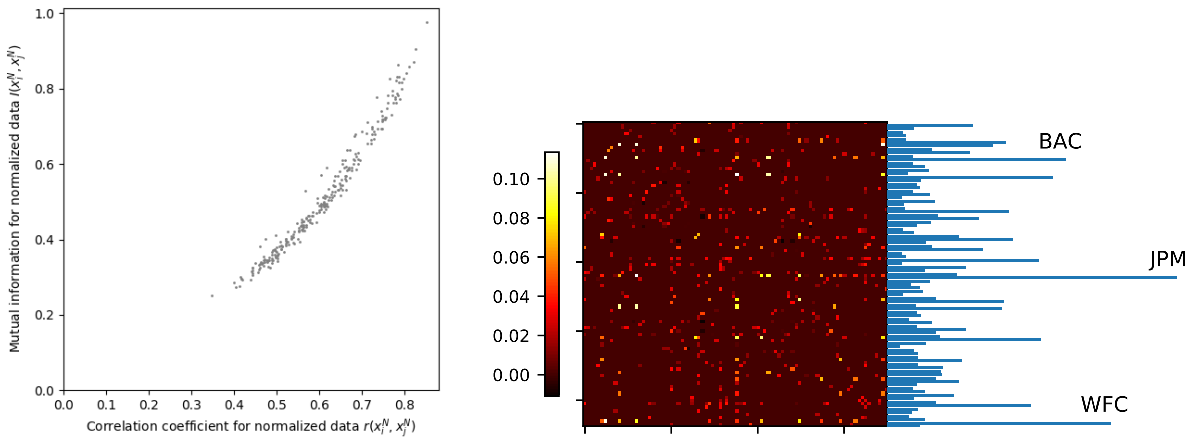


Figure 5: *Left*: Relation between correlation and mutual information estimates from the normalized filtered data, i.e. only those later used for PMFG construction, having original setting similar as in Figure 2. *Right*: Extranormal information $I_e$ for normalized filtered data with summed rows and highlighted extremes.

We present again the most influencing stocks from viewpoint of nonlinear contribution within the original scatter plot of mutual information and correlation, see Figure 6.

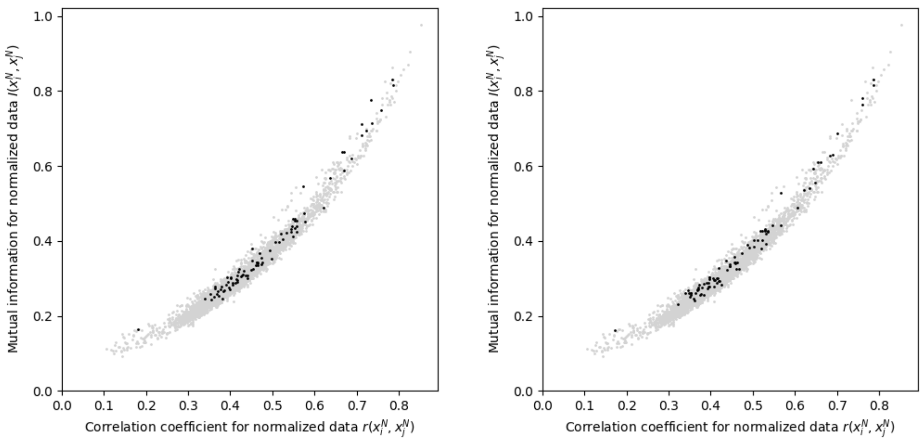


Figure 6: Relation between correlation and mutual information estimates computed from the normalized data having similar setting as in Figure 2 with one chosen highlighted stock in black. *Left*: the JPM stock . *Right*: the WFC stock.

Removing some of the stocks given by analysis of nonlinearity strongest sources in data given by PMFG and MST filterings, see above, we can compare linear and nonlinear contribution at the level of global network characteristics, see Figure 7.

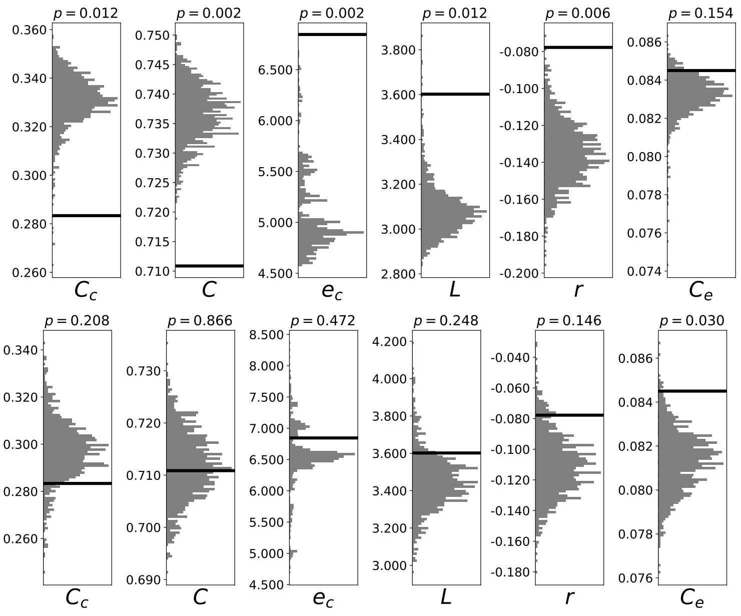


(a) Network from original data with stocks AIG, F, JPM and WFC removed and filtered using PMFG

(b) Network from marginally normalized data with stocks AIG, F, JPM and WFC removed and network filtered using PMFG

Figure 7: Global graph characteristics computed for networks constructed out of real data (blue bullets) and out of linearized surrogate datasets (gray bullets) both based on the NYSE100 index with different sets of stocks removed. Connectivity has been computed using mutual information for original and marginally normalized data augmented with 99 linear surrogates. Presented characteristics are closeness $C_c$, average clustering coefficient $C$, eccentricity $e_C$, average shortest path $L$, assortative coefficient $r$ and eigenvalue centrality $C_e$.

Figure 8 contains results of nonlinearity analysis for networks using the WTA filtering.

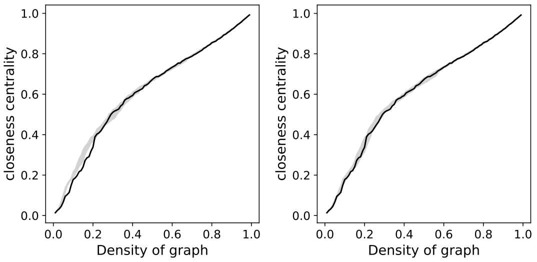


(a) Closeness centrality

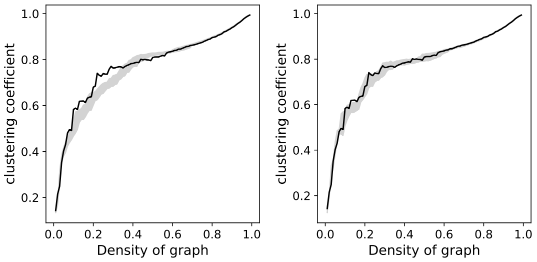


(b) Clustering coefficient

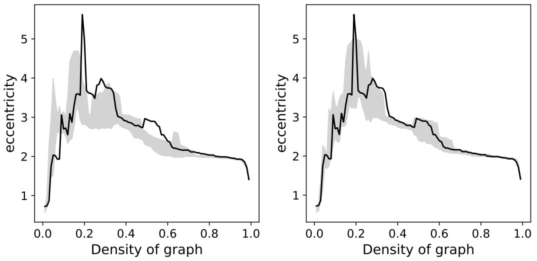


(c) Eccentricity

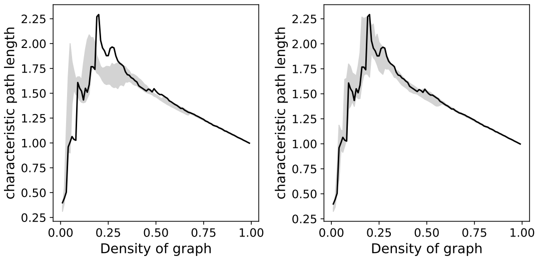


(d) Characteristic path length

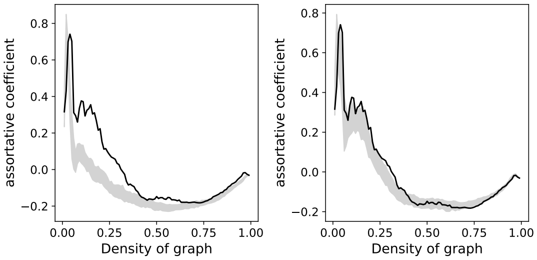


(e) Assortative coefficient

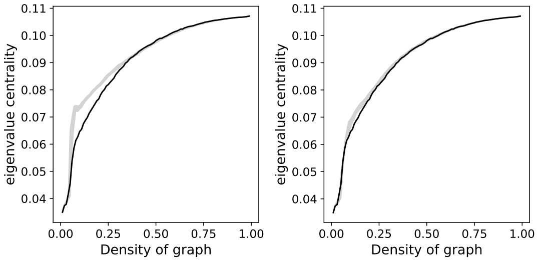


(f) Eigenvector centrality

Figure 8: Global graph characteristics each one plotted as a function of density of network determined via the WTA filtering across a range of densities from 0 to 0.99 with a step of 0.01 computed for data and 99 linear surrogates. Plots are data derived networks (black lines) and gray area representing interval of plots of linearized surrogate datasets (gray area). Considered network is constructed out of stocks from NYSE100 index with stock AIG removed where connectivity has been determined via mutual information without any normalization (left figures) and with unvariatelly normalization applied (right figures). For mutual information estimates binning parameter were 8.

# 3 FTSE100 index

This section contains results for stocks in the FTSE100 index with the same settings of analysis as presented in the main body of work. At first, stocks considered in FTSE100 index is listed in Table 2. This table is followed by Figure 9 showing FTSE100 stocks existence within considered period. What follows are results showing nonlinearity assessment within FTSE100 index.

Table 2: Table of considered companies as part of stocks index FTSE100 that were traded between 11 November 2003 and 7 November 2013.

| | | | |
|---|---|---|---|
| III.L | 3i Group | LGEN.L | Legal & General Group |
| ABF.L | Associated British Foods | LLOY.L | Lloyds Banking Group |
| AAL.L | Anglo American | LSE.L | London Stock Exchange Group |
| ANTO.L | Antofagasta | MKS.L | Marks & Spencer Group |
| AHT.L | Ashtead Group | MRW.L | Morrison (Wm) Supermarkets |
| AZN.L | AstraZeneca | NG.L | National Grid |
| AV.L | Aviva | NXT.L | Next |
| BAB.L | Babcock International Group | OML.L | Old Mutual |
| BA.L | BAE Systems | PPB.L | Paddy Power Betfair |
| BARC.L | Barclays | PSON.L | Pearson |
| BDEV.L | Barratt Developments | PSN.L | Persimmon |
| BKG.L | Berkeley Group Holdings | PRU.L | Prudential |
| BLT.L | BHP Billiton | RRS.L | Randgold Resources |
| BP.L | BP | RDSB.L | Royal Dutch Shell B |
| BATS.L | British American Tobacco | RB.L | Reckitt Benckiser Group |
| BLND.L | British Land Co | REL.L | RELX |
| BT | BT Group | RTO.L | Rentokil Initial |
| BNZL.L | Bunzl | RIO.L | Rio Tinto |
| BRBY.L | Burberry Group | RR.L | Rolls-Royce Holdings |
| CCL.L | Carnival | RBS.L | Royal Bank Of Scotland Group |
| CNA.L | Centrica | RSA.L | RSA Insurance Group |
| CPG.L | Compass Group | SGE.L | Sage Group |
| CRH.L | CRH | SBRY.L | Sainsbury (J) |
| CRDA.L | Croda International | SDR.L | Schroders |
| DCC.L | DCC | SMT.L | Scottish Mortgage Inv Tst |
| DGE.L | Diageo | SGRO.L | Segro |
| EZJ.L | Easyjet | SVT.L | Severn Trent |
| GFS.L | G4S | SHP.L | Shire |
| GKN.L | GKN | SKY.L | Sky |
| GSK.L | GlaxoSmithKline | SN.L | Smith & Nephew |
| HMSO.L | Hammerson | SMIN.L | Smiths Group |
| HSBA.L | HSBC Hldgs | SSE.L | SSE |
| IMB.L | Imperial Brands | STJ.L | St. James's Place |
| INF.L | Informa | STAN.L | Standard Chartered |
| IHG.L | InterContinental Hotels Group | TW.L | Taylor Wimpey |
| ITRK.L | Intertek Group | TSCO.L | Tesco |
| IAG.L | Internat. Consolidated Airlines Group | ULVR.L | Unilever |
| ITV.L | ITV | UU.L | United Utilities Group |
| JMAT.L | Johnson Matthey | VOD.L | Vodafone Group |
| KGF.L | Kingfisher | WTB.L | Whitbread |
| LAND.L | Land Securities Group | WPP.L | WPP |

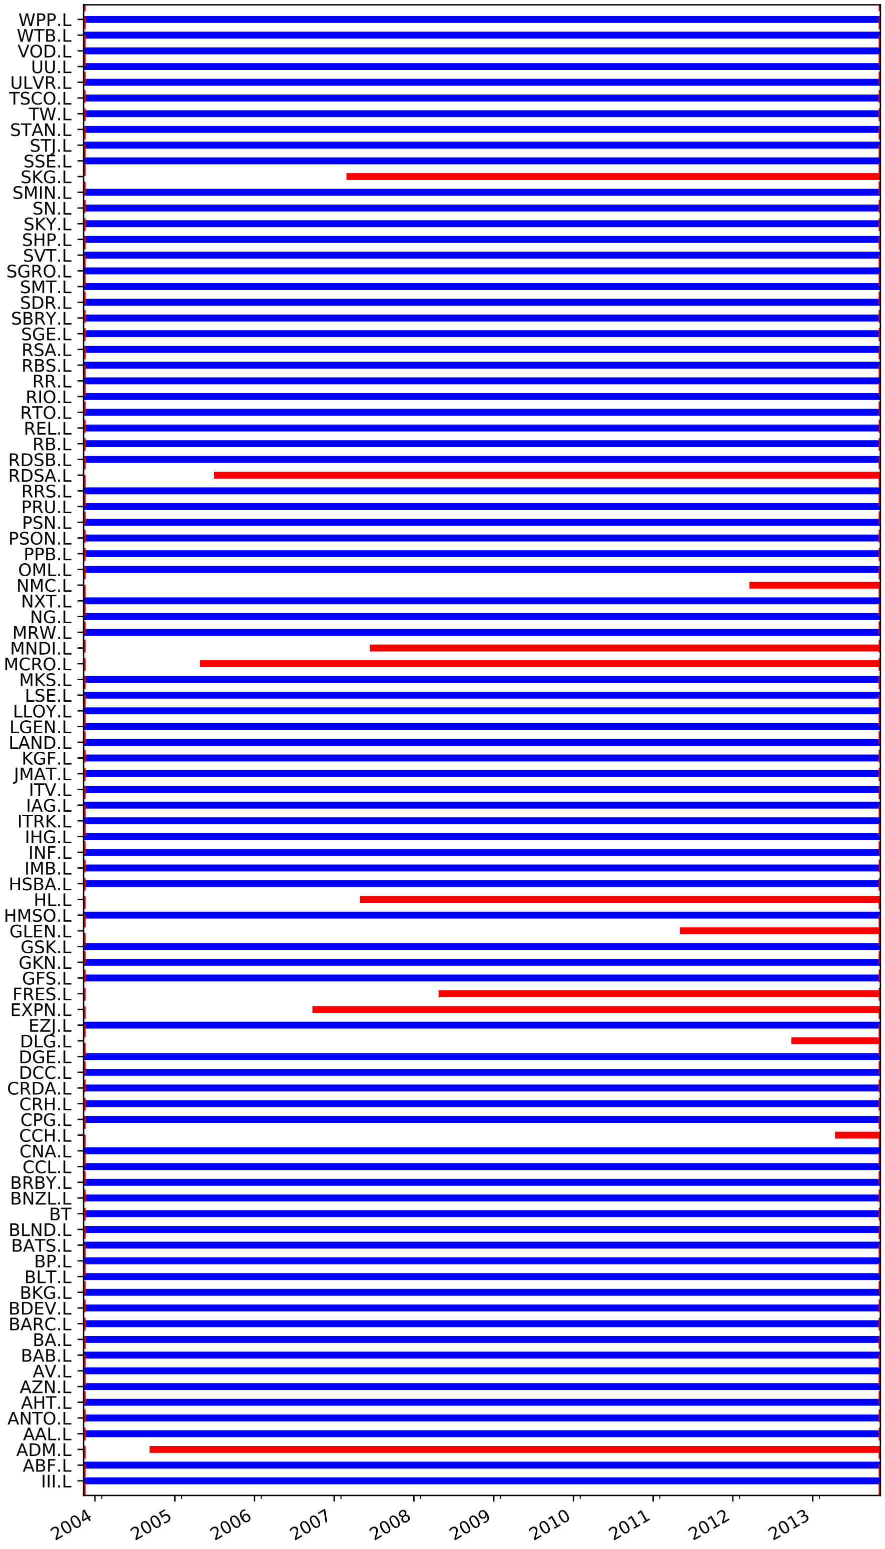


Figure 9: Plot showing existence intervals for stocks from FTSE100 index. Those traded between 11 November 2003 and 7 November 2013 are indicated blue, while others with shorter interval of existence are denoted as red.

## 3.1 Analysis of nonlinearity of stocks network for FTSE100

This section presents results of the analysis with the original setting. Relation between values of correlation coefficient and mutual informations are shown in Figure 10.

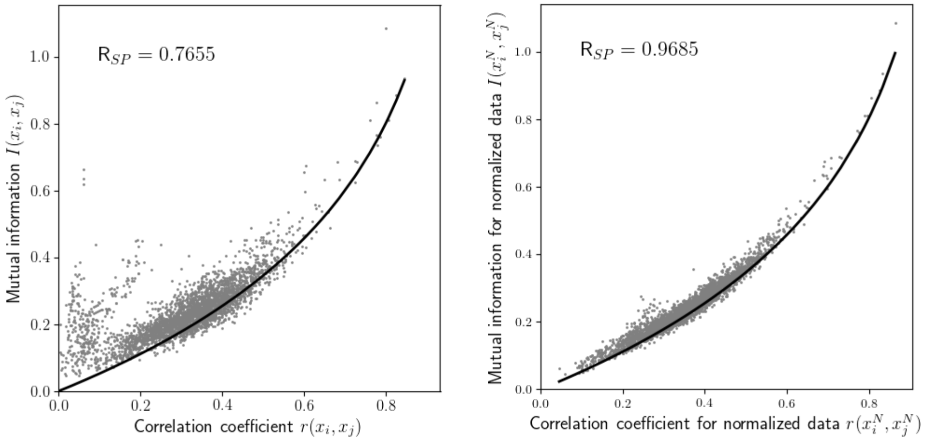


Figure 10: Relation between correlation and mutual information estimates from the original data (left) and marginally normalized data (right). Original data were log-returns of the close prices of the FTSE100 stocks traded between 11 November 2003 and 7 November 2013. To estimate mutual information 4 bins are used for discretization. Each gray point represents the values of $r(x_i, x_j)$ and $I(x_i, x_j)$ (left) or $r(x_i^N, x_j^N)$ and $I(x_i^N, x_j^N)$ (right) for a pair of variables $x_i, x_j$ (left) or $x_i^N, x_j^N$ (right) for $i, j \in \{1, \ldots, N\}$. Gaussian mutual information $I_G$ shown by black line.

Localization of remaining nonlinearity after normalization is presented in Figure 11 providing detection of a stock with the highest contribution and its further visualization.

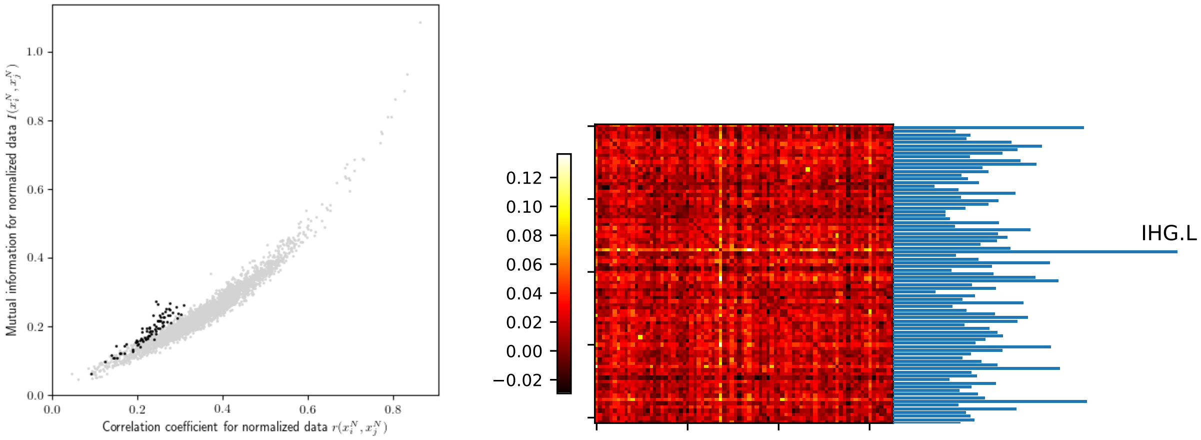


Figure 11: *Right*: Relation between correlation and mutual information estimates from the normalized data having similar setting as in Figure 10 with stock IHG.L highlighted in black. *Left*: Extranormal information $I_e$ for normalized data with summed rows and highlighted extremes.

With stock IHG.L removed further comparison of linear and nonlinear contribution can be done at the level of global network characteristics. Results are shown in Figure 12.

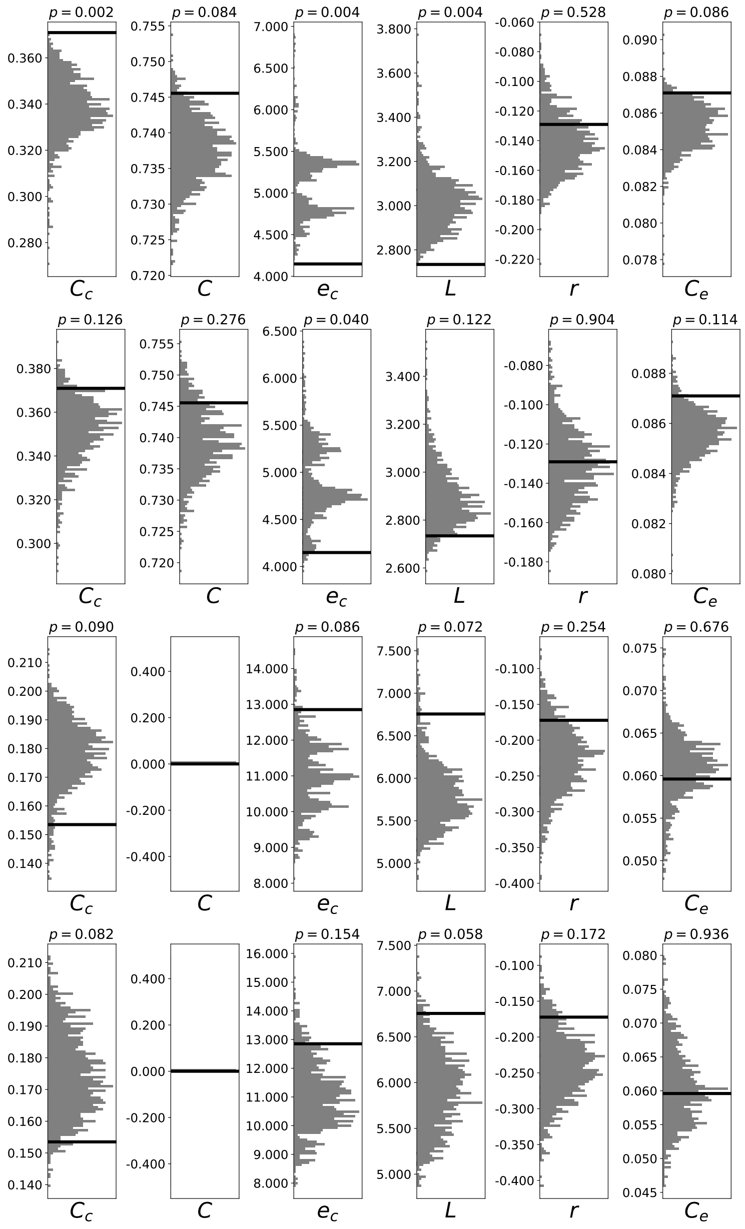


(a) Network from original data filtered using PMFG

(b) Network from marginally normalized data filtered using PMFG

(c) Network from original data filtered using MST

(d) Network from marginally normalized data filtered using MST

Figure 12: Global graph characteristics computed for networks constructed out of real data (blue bullets) and out of linearized surrogate datasets (gray bullets) both based on the FTSE100 index with the stock IHG.L removed. Connectivity has been computed using mutual information for original and marginally normalized data augmented with 99 linear surrogates. Presented characteristics are closeness $C_c$, average clustering coefficient $C$, eccentricity $e_C$, average shortest path $L$, assortative coefficient $r$ and eigenvalue centrality $C_e$.

For networks constructed using the MST filtering nonlinearity seems not to play a significant role. On the other hand, for networks constructed using the PMFG filtering eccentricity seems to be on the boundary of linear results, see Figure 12. In this case it is necessary to explore possible sources in more detail. Instead of analyzing extranormal information for all pairs as in Figure 11 we filter out only pairs responsible for PMFG network construction and analyze their contribution, see Figure 13.

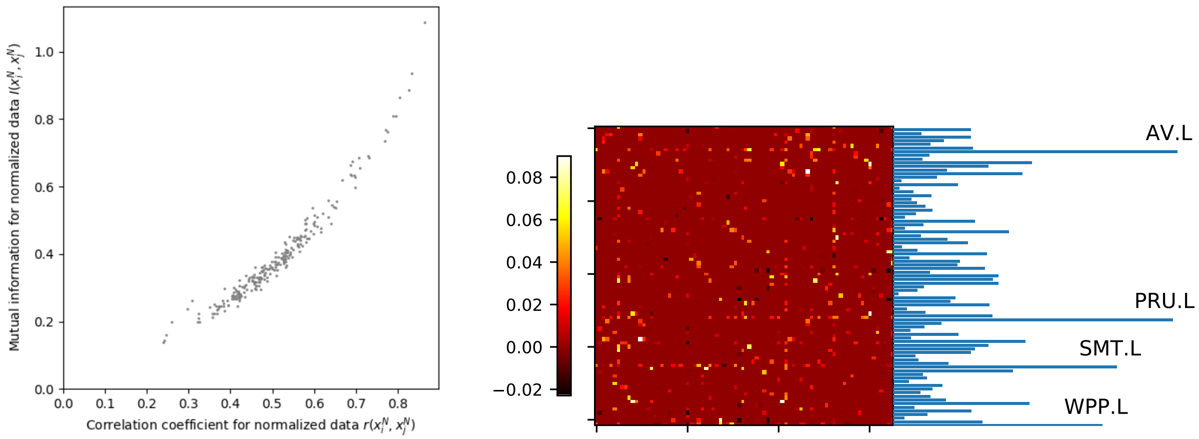


Figure 13: *Right*: Relation between correlation and mutual information estimates from the normalized filtered data data, i.e. only those later used for PMFG construction, having original setting similar as in Figure 10. *Left*: Extranormal information $I_e$ for normalized filtered data with summed rows and highlighted extremes.

We present most influencing stocks from viewpoint of nonlinear contribution within the original scatter plot of mutual information and correlation, see Figure 14.

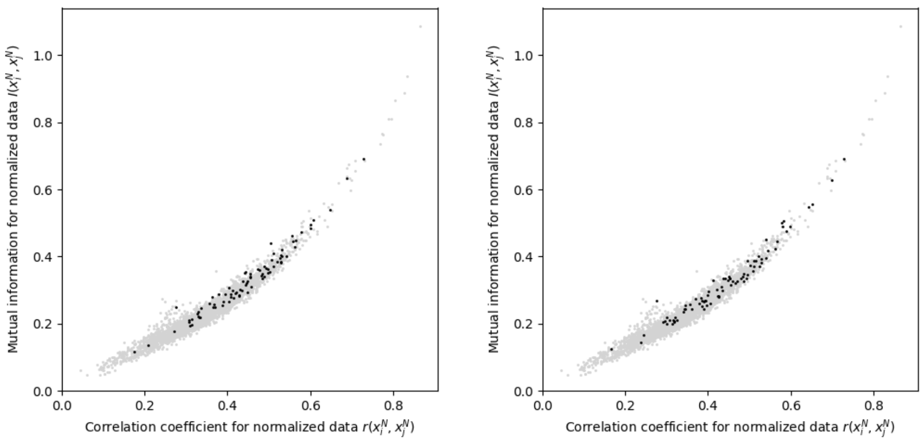

Figure 14: Relation between correlation and mutual information estimates computed from the normalized data having similar setting as in Figure 10 with one chosen highlighted stock in black. *Right*: the PRU.L stock . *Left*: the AV.L stock.

With stocks IHG.L, PRU.L, and AV.L removed further comparison of linear and nonlinear contribution can be done at the level of global network characteristics. Results are shown in Figure 15.

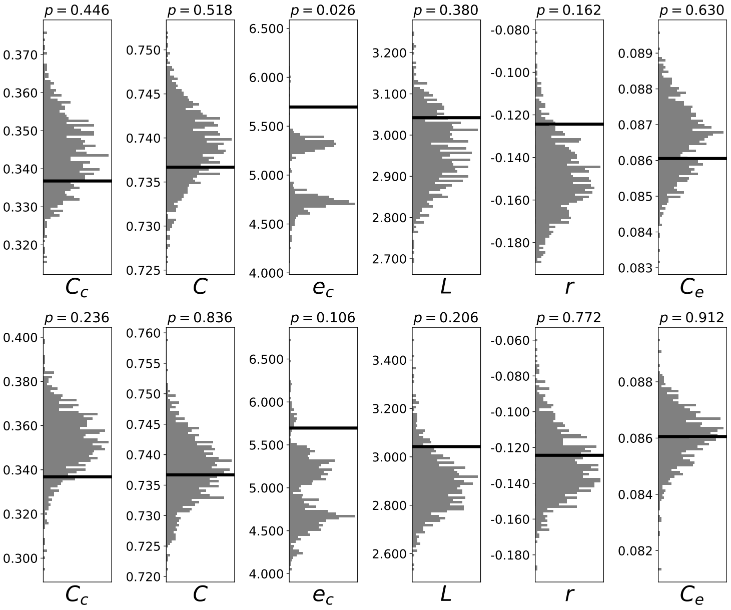


(a) Network from original data with stocks IHG.L, PRU.L and AV.L removed and filtered using PMFG

(b) Network from marginally normalized data with stocks IHG.L, PRU.L and AV.L removed and network filtered using PMFG

Figure 15: Global graph characteristics computed for networks constructed out of real data (blue bullets) and out of linearized surrogate datasets (gray bullets) both based on the FTSE100 index with the stocks IHG.L, PRU.L and AV.L removed. Connectivity has been computed using mutual information for original (above) and marginally normalized (below) data augmented with 99 linear surrogates. Presented characteristics are closeness $C_c$, average clustering coefficient $C$, eccentricity $e_C$, average shortest path $L$, assortative coefficient $r$ and eigenvalue centrality $C_e$.

Figure 16 contains results of nonlinearity analysis for networks using the WTA filtering.

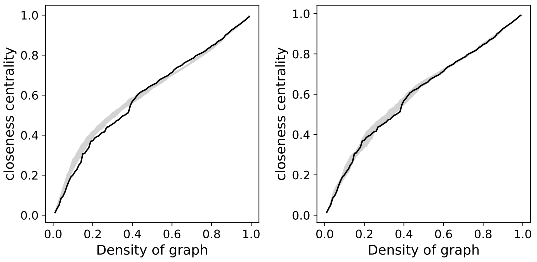


(a) Closeness centrality

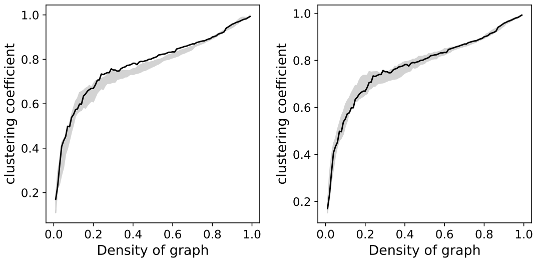


(b) Clustering coefficient

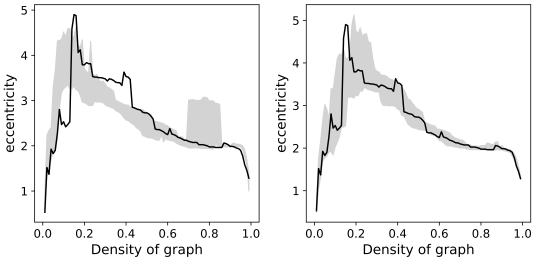


(c) Eccentricity

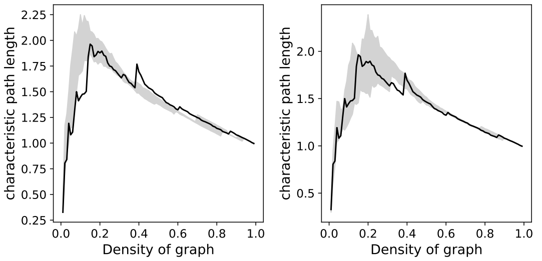


(d) Characteristic path length

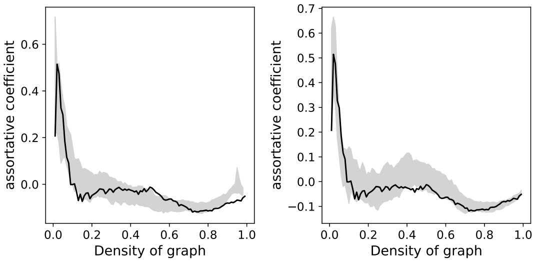


(e) Assortative coefficient

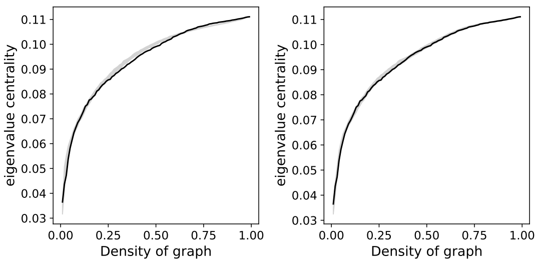


(f) Eigenvector centrality

Figure 16: Values of global graph characteristics each one plotted as function of density of network determined via winner-takes-all filtering across a range of densities from 0 to 0.99 with a step of 0.01. There were 99 linear surrogates for which the same analysis has been computed. Plots are data derived networks (black lines) and gray area representing interval of plots of linearized surrogate datasets (gray area). Considered network is constructed out of stocks from FTSE100 index with stock IHG.L removed where connectivity has been determined via mutual information without any normalization (left) and with unvariatelly normalization applied (right). We use stocks traded between 11 November 2003 and 7 November 2013 and mutual information estimates have binning parameter equal to 4.

# 4 SP500 index

This section contains results for analysis, with the original settings, of stocks from SP500 index. Stocks considered for the analysis are shown in Tables 3, 4, 5, 6, 7. Only 405 considered stocks traded between 11 November 2003 and 7 November 2013 from SP500 are considered and shown. That is why long figure showing filtering strategy for all remaining 95 stocks, e.g. Figure 1, is not presented.

Table 3: Table of all 405 considered companies as part of stocks index SP500. First 81 companies

| | | | |
|---|---|---|---|
| PCLN | Priceline Group Inc/The | BDX | Becton Dickinson and Co |
| AZO | AutoZone Inc | SRCL | Stericycle Inc |
| ISRG | Intuitive Surgical Inc | HSIC | Henry Schein Inc |
| NFLX | Netflix Inc | MLM | Martin Marietta Materials Inc |
| REGN | Regeneron Pharmaceuticals Inc | BXP | Boston Properties Inc |
| BIIB | Biogen Inc | RL | Ralph Lauren Corp |
| AMZN | Amazon.com Inc | CMI | Cummins Inc |
| BLK | BlackRock Inc | MNST | Monster Beverage Corp |
| ADS | Alliance Data Systems Corp | GD | General Dynamics Corp |
| SHW | Sherwin-Williams Co/The | CI | Cigna Corp |
| EQIX | Equinix Inc | TMO | Thermo Fisher Scientific Inc |
| GWW | WW Grainger Inc | DNB | Dun & Bradstreet Corp/The |
| PPG | PPG Industries Inc | VRTX | Vertex Pharmaceuticals Inc |
| MCK | McKesson Corp | SLG | SL Green Realty Corp |
| ESS | Essex Property Trust Inc | WYNN | Wynn Resorts Ltd |
| AMG | Affiliated Managers Group Inc | XEC | Cimarex Energy Co |
| ORLY | O'Reilly Automotive Inc | AAPL | Apple Inc |
| PRGO | Perrigo Co PLC | WAT | Waters Corp |
| GS | Goldman Sachs Group Inc/The | LH | Laboratory Corp of America Holdings |
| LMT | Lockheed Martin Corp | LLL | L-3 Communications Holdings Inc |
| WHR | Whirlpool Corp | MTB | M&T Bank Corp |
| PSA | Public Storage | PH | Parker-Hannifin Corp |
| SPG | Simon Property Group Inc | PX | Praxair Inc |
| MHK | Mohawk Industries Inc | UNH | UnitedHealth Group Inc |
| ALXN | Alexion Pharmaceuticals Inc | UHS | Universal Health Services Inc |
| HUM | Humana Inc | MON | Monsanto Co |
| PXD | Pioneer Natural Resources Co | IFF | International Flavors & Fragrances Inc |
| FDX | FedEx Corp | STZ | Constellation Brands Inc |
| BCR | CR Bard Inc | SJM | JM Smucker Co/The |
| ROP | Roper Industries Inc | UTX | United Technologies Corp |
| AVB | AvalonBay Communities Inc | ECL | Ecolab Inc |
| MMM | 3M Co | CELG | Celgene Corp |
| NOC | Northrop Grumman Corp | HD | Home Depot Inc/The |
| AMGN | Amgen Inc | ABC | AmerisourceBergen Corp |
| IBM | International Business Machines Corp | FFIV | F5 Networks Inc |
| ANTM | Anthem Inc | ROK | Rockwell Automation Inc |
| BA | Boeing Co/The | CLX | Clorox Co/The |
| APD | Air Products & Chemicals Inc | PVH | PVH Corp |
| COST | Costco Wholesale Corp | CVX | Chevron Corp |
| SNA | Snap-on Inc | RTN | Raytheon Co |
| EW | Edwards Lifesciences Corp | | |

Table 4: Table of all 405 considered companies as part of stocks index SP500. Second 81 companies.

| | | | |
|---|---|---|---|
| SRE | Sempra Energy | WBA | Walgreens Boots Alliance Inc |
| VNO | Vornado Realty Trust | CME | CME Group Inc/IL |
| UNP | Union Pacific Corp | APC | Anadarko Petroleum Corp |
| AET | Aetna Inc | CAH | Cardinal Health Inc |
| TRV | Travelers Cos Inc/The | SLB | Schlumberger Ltd |
| KMB | Kimberly-Clark Corp | ESRX | Express Scripts Holding Co |
| DIS | Walt Disney Co/The | DE | Deere & Co |
| KSU | Kansas City Southern | TIF | Tiffany & Co |
| MCO | Moody's Corp | TSCO | Tractor Supply Co |
| NEE | NextEra Energy Inc | XOM | Exxon Mobil Corp |
| ROST | Ross Stores Inc | ADP | Automatic Data Processing Inc |
| HON | Honeywell International Inc | DHR | Danaher Corp |
| GILD | Gilead Sciences Inc | CCI | Crown Castle International Corp |
| CVS | CVS Health Corp | EL | Estee Lauder Cos Inc/The |
| CB | Chubb Corp/The | EQT | EQT Corp |
| HSY | Hershey Co/The | TWX | Time Warner Inc |
| JNJ | Johnson & Johnson | PG | Procter & Gamble Co/The |
| NSC | Norfolk Southern Corp | VMC | Vulcan Materials Co |
| NKE | NIKE Inc | TGT | Target Corp |
| ITW | Illinois Tool Works Inc | CAT | Caterpillar Inc |
| AON | Aon PLC | TROW | T Rowe Price Group Inc |
| INTU | Intuit Inc | DVA | DaVita HealthCare Partners Inc |
| COL | Rockwell Collins Inc | CTAS | Cintas Corp |
| MCD | McDonald's Corp | DTE | DTE Energy Co |
| URI | United Rentals Inc | COF | Capital One Financial Corp |
| UPS | United Parcel Service Inc | MAC | Macerich Co/The |
| PEP | PepsiCo Inc | FOSL | Fossil Group Inc |
| EOG | EOG Resources Inc | DLTR | Dollar Tree Inc |
| WDC | Western Digital Corp | HRS | Harris Corp |
| SWK | Stanley Black & Decker Inc | WMT | Wal-Mart Stores Inc |
| SWKS | Skyworks Solutions Inc | RCL | Royal Caribbean Cruises Ltd |
| R | Ryder System Inc | PRU | Prudential Financial Inc |
| AMT | American Tower Corp | YUM | Yum! Brands Inc |
| VAR | Varian Medical Systems Inc | AXP | American Express Co |
| EFX | Equifax Inc | OXY | Occidental Petroleum Corp |
| ACN | Accenture PLC | MAR | Marriott International Inc/MD |
| LB | L Brands Inc | JWN | Nordstrom Inc |
| PNC | PNC Financial Services Group Inc/The | FISV | Fiserv Inc |
| ENDP | Endo International PLC | OMC | Omnicom Group Inc |
| GPC | Genuine Parts Co | MDT | Medtronic PLC |
| SYK | Stryker Corp | | |

Table 5: Table of all 405 considered companies as part of stocks index SP500. Third 81 companies.

| | | | |
|---|---|---|---|
| MKC | McCormick & Co Inc/MD | VRSN | VeriSign Inc |
| ETR | Entergy Corp | TJX | TJX Cos Inc/The |
| DUK | Duke Energy Corp | DVN | Devon Energy Corp |
| TAP | Molson Coors Brewing Co | K | Kellogg Co |
| KSS | Kohl's Corp | AN | AutoNation Inc |
| STT | State Street Corp | AFL | Aflac Inc |
| HCN | Health Care REIT Inc | HAS | Hasbro Inc |
| EQR | Equity Residential | FIS | Fidelity National Information Services I |
| ADBE | Adobe Systems Inc | BMY | Bristol-Myers Squibb Co |
| HP | Helmerich & Payne Inc | CTXS | Citrix Systems Inc |
| KR | Kroger Co/The | PNR | Pentair PLC |
| RHT | Red Hat Inc | PNW | Pinnacle West Capital Corp |
| VFC | VF Corp | PCAR | PACCAR Inc |
| HES | Hess Corp | JPM | JPMorgan Chase & Co |
| DGX | Quest Diagnostics Inc | EIX | Edison International |
| LOW | Lowe's Cos Inc | CTSH | Cognizant Technology Solutions Corp |
| VTR | Ventas Inc | ADI | Analog Devices Inc |
| CERN | Cerner Corp | HOG | Harley-Davidson Inc |
| LLY | Eli Lilly & Co | ADSK | Autodesk Inc |
| BBBY | Bed Bath & Beyond Inc | MSI | Motorola Solutions Inc |
| EMN | Eastman Chemical Co | ED | Consolidated Edison Inc |
| BLL | Ball Corp | BWA | BorgWarner Inc |
| KMX | CarMax Inc | KLAC | KLA-Tencor Corp |
| DD | EI du Pont de Nemours & Co | RHI | Robert Half International Inc |
| LRCX | Lam Research Corp | FLR | Fluor Corp |
| D | Dominion Resources Inc/VA | CMCSA | Comcast Corp |
| ALL | Allstate Corp/The | APH | Amphenol Corp |
| NTRS | Northern Trust Corp | FMC | FMC Corp |
| AKAM | Akamai Technologies Inc | EMR | Emerson Electric Co |
| DOV | Dover Corp | HRL | Hormel Foods Corp |
| CHRW | CH Robinson Worldwide Inc | MRK | Merck & Co Inc |
| BAX | Baxter International Inc | RRC | Range Resources Corp |
| APA | Apache Corp | AIG | American International Group Inc |
| CL | Colgate-Palmolive Co | MMC | Marsh & McLennan Cos Inc |
| QCOM | QUALCOMM Inc | VLO | Valero Energy Corp |
| ETN | Eaton Corp PLC | EA | Electronic Arts Inc |
| MYL | Mylan NV | EBAY | eBay Inc |
| IR | Ingersoll-Rand PLC | TXN | Texas Instruments Inc |
| COP | ConocoPhillips | GIS | General Mills Inc |
| M | Macy's Inc | LNC | Lincoln National Corp |
| DRI | Darden Restaurants Inc | | |

Table 6: Table of all 405 considered companies as part of stocks index SP500. Fourth 81 companies.

| | | | |
|---|---|---|---|
| AEP | American Electric Power Co Inc | CCL | Carnival Corp |
| TMK | Torchmark Corp | GRMN | Garmin Ltd |
| FLS | Flowserve Corp | EXPD | Expeditors International of Washington I |
| STX | Seagate Technology PLC | JEC | Jacobs Engineering Group Inc |
| IP | International Paper Co | ABT | Abbott Laboratories |
| SCG | SCANA Corp | CPB | Campbell Soup Co |
| NOV | National Oilwell Varco Inc | HAL | Halliburton Co |
| LM | Legg Mason Inc | TXT | Textron Inc |
| WM | Waste Management Inc | MOS | Mosaic Co/The |
| WFC | Wells Fargo & Co | CMA | Comerica Inc |
| CINF | Cincinnati Financial Corp | LEG | Leggett & Platt Inc |
| AVY | Avery Dennison Corp | SEE | Sealed Air Corp |
| AME | AMETEK Inc | CCE | Coca-Cola Enterprises Inc |
| LVLT | Level 3 Communications Inc | SO | Southern Co/The |
| C | Citigroup Inc | URBN | Urban Outfitters Inc |
| PCG | PG&E Corp | USB | US Bancorp/MN |
| BEN | Franklin Resources Inc | NI | NiSource Inc |
| MO | Altria Group Inc | XLNX | Xilinx Inc |
| NBL | Noble Energy Inc | A | Agilent Technologies Inc |
| XRAY | DENTSPLY International Inc | PLD | Prologis Inc |
| PKI | PerkinElmer Inc | ORCL | Oracle Corp |
| PFG | Principal Financial Group Inc | HCP | HCP Inc |
| LEN | Lennar Corp | HIG | Hartford Financial Services Group Inc/Th |
| THC | Tenet Healthcare Corp | LUV | Southwest Airlines Co |
| WMB | Williams Cos Inc/The | COH | Coach Inc |
| MET | MetLife Inc | FAST | Fastenal Co |
| ES | Eversource Energy | AEE | Ameren Corp |
| O | Realty Income Corp | MSFT | Microsoft Corp |
| JCI | Johnson Controls Inc | L | Loews Corp |
| WEC | Wisconsin Energy Corp | STI | SunTrust Banks Inc |
| NDAQ | NASDAQ OMX Group Inc/The | PEG | Public Service Enterprise Group Inc |
| MUR | Murphy Oil Corp | GPS | Gap Inc/The |
| OKE | ONEOK Inc | BK | Bank of New York Mellon Corp/The |
| VZ | Verizon Communications Inc | KO | Coca-Cola Co/The |
| PAYX | Paychex Inc | GME | GameStop Corp |
| DOW | Dow Chemical Co/The | IVZ | Invesco Ltd |
| MCHP | Microchip Technology Inc | RSG | Republic Services Inc |
| SBUX | Starbucks Corp | TSN | Tyson Foods Inc |
| PDCO | Patterson Cos Inc | NWL | Newell Rubbermaid Inc |
| ADM | Archer-Daniels-Midland Co | BBT | BB&T Corp |
| NUE | Nucor Corp | | |

Table 7: Table of all 405 considered companies as part of stocks index SP500. Fifth 81 companies.

| | | | |
|---|---|---|---|
| FTI | FMC Technologies Inc | GE | General Electric Co |
| AIV | Apartment Investment & Management Co | MU | Micron Technology Inc |
| XL | XL Group PLC | ZION | Zions Bancorporation |
| TSS | Total System Services Inc | GT | Goodyear Tire & Rubber Co/The |
| BBY | Best Buy Co Inc | PGR | Progressive Corp/The |
| SYY | Sysco Corp | MAS | Masco Corp |
| CAG | ConAgra Foods Inc | KIM | Kimco Realty Corp |
| MDLZ | Mondelez International Inc | SWN | Southwestern Energy Co |
| NFX | Newfield Exploration Co | ESV | Ensco PLC |
| IRM | Iron Mountain Inc | MAT | Mattel Inc |
| MS | Morgan Stanley | OI | Owens-Illinois Inc |
| GCI | Gannett Co Inc | JNPR | Juniper Networks Inc |
| NTAP | NetApp Inc | SYMC | Symantec Corp |
| FE | FirstEnergy Corp | PBI | Pitney Bowes Inc |
| CTL | CenturyLink Inc | LUK | Leucadia National Corp |
| PFE | Pfizer Inc | NEM | Newmont Mining Corp |
| CMS | CMS Energy Corp | PHM | PulteGroup Inc |
| XEL | Xcel Energy Inc | NVDA | NVIDIA Corp |
| FOXA | Twenty-First Century Fox Inc | GLW | Corning Inc |
| PPL | PPL Corp | AMAT | Applied Materials Inc |
| UNM | Unum Group | IPG | Interpublic Group of Cos Inc/The |
| EXC | Exelon Corp | CNP | CenterPoint Energy Inc |
| CSX | CSX Corp | HST | Host Hotels & Resorts Inc |
| T | AT&T Inc | FITB | Fifth Third Bancorp |
| HPQ | Hewlett-Packard Co | FCX | Freeport-McMoRan Inc |
| WY | Weyerhaeuser Co | BSX | Boston Scientific Corp |
| HRB | H&R Block Inc | RIG | Transocean Ltd |
| COG | Cabot Oil & Gas Corp | NE | Noble Corp plc |
| INTC | Intel Corp | SPLS | Staples Inc |
| CA | CA Inc | F | Ford Motor Co |
| FLIR | FLIR Systems Inc | BAC | Bank of America Corp |
| DO | Diamond Offshore Drilling Inc | CHK | Chesapeake Energy Corp |
| ATI | Allegheny Technologies Inc | PBCT | People's United Financial Inc |
| SCHW | Charles Schwab Corp/The | KEY | KeyCorp |
| MRO | Marathon Oil Corp | AA | Alcoa Inc |
| PWR | Quanta Services Inc | AES | AES Corp/VA |
| GGP | General Growth Properties Inc | XRX | Xerox Corp |
| DHI | DR Horton Inc | HBAN | Huntington Bancshares Inc/OH |
| CNX | CONSOL Energy Inc | RF | Regions Financial Corp |
| ETFC | E*TRADE Financial Corp | FTR | Frontier Communications Corp |
| CSCO | Cisco Systems Inc | | |

## 4.1 Analysis of nonlinearity

This section presents results of the analysis with the original setting. Relation between values of correlation coefficient and mutual informations are shown in Figure 17.

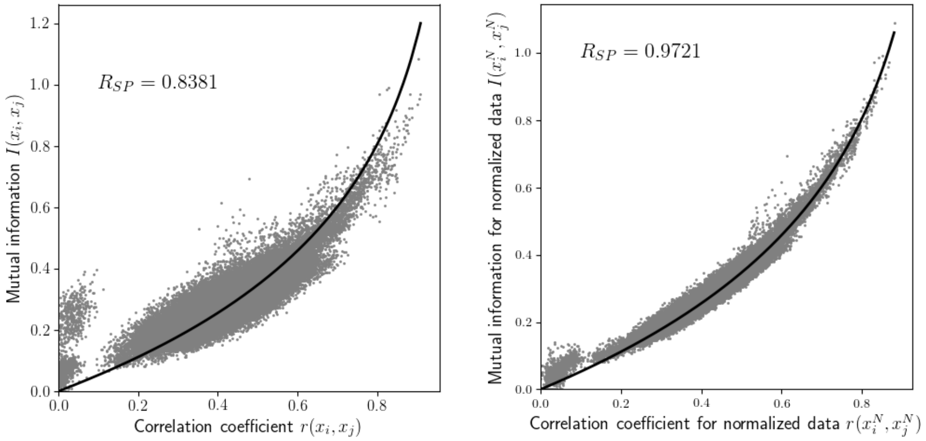


Figure 17: Relation between correlation and mutual information estimates from the original data (left) and marginally normalized data (right). Original data were log-returns of the close prices of the SP500 stocks. To estimate mutual information 4 bins were used. Each gray point represents the values of $r(x_i, x_j)$ and $I(x_i, x_j)$ (left) or $r(x_i^N, x_j^N)$ and $I(x_i^N, x_j^N)$ (right) for a pair $x_i, x_j$ (left) or $x_i^N, x_j^N$ (right) for $i, j \in \{1, \ldots, N\}$. Gaussian mutual information $I_G$ shown in black.

Localization of remaining nonlinearity after normalization is presented in Figure 18.

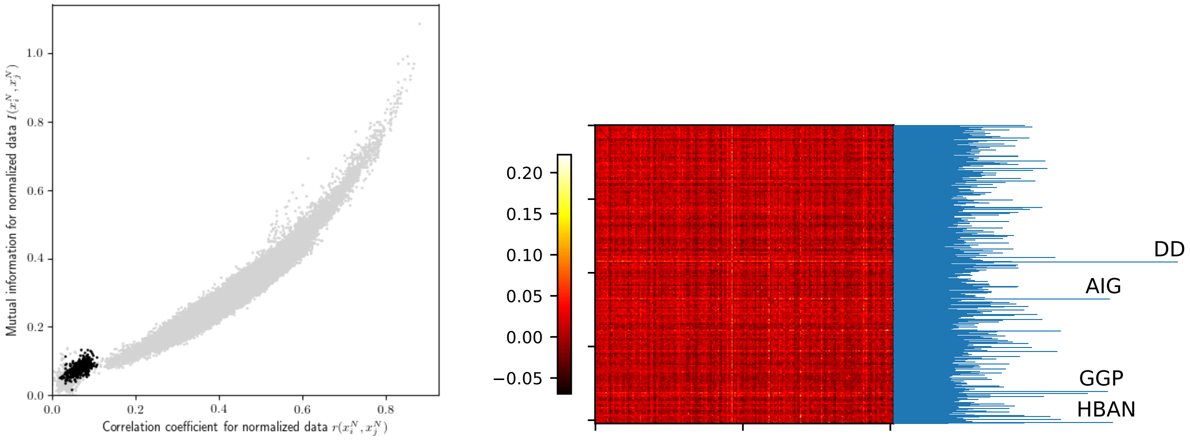


Figure 18: *Right*: Relation between correlation and mutual information estimates from the normalized data having similar setting as in Figure 17 with stock DD highlighted in black. *Left*: Extranormal information $I_e$ for normalized data with summed rows and highlighted extremes.

With stock DD removed further comparison of linear and nonlinear contribution can be done at the level of global network characteristics. Results are shown in Figure 19.

For networks constructed using PMFG filtering nonlinearity seems to play a significant role, especially characteristics based on path lengths are influenced, see Figure 19. In this case it is necessary to explore possible sources in more detail. We filter out only pairs responsible for PMFG network construction and analyze their contribution, see Figure 20.

For the most influencing stocks from viewpoint of nonlinear contribution shown in original scatter see Figure 21.

With stocks DD, TROW and ADI removed further comparison of linear and nonlinear contribution can be done at the level of global network characteristics. Results are shown in Figure 22 presenting values of global graph characteristics for networks constructed out of original data as well as marginally normalized data.

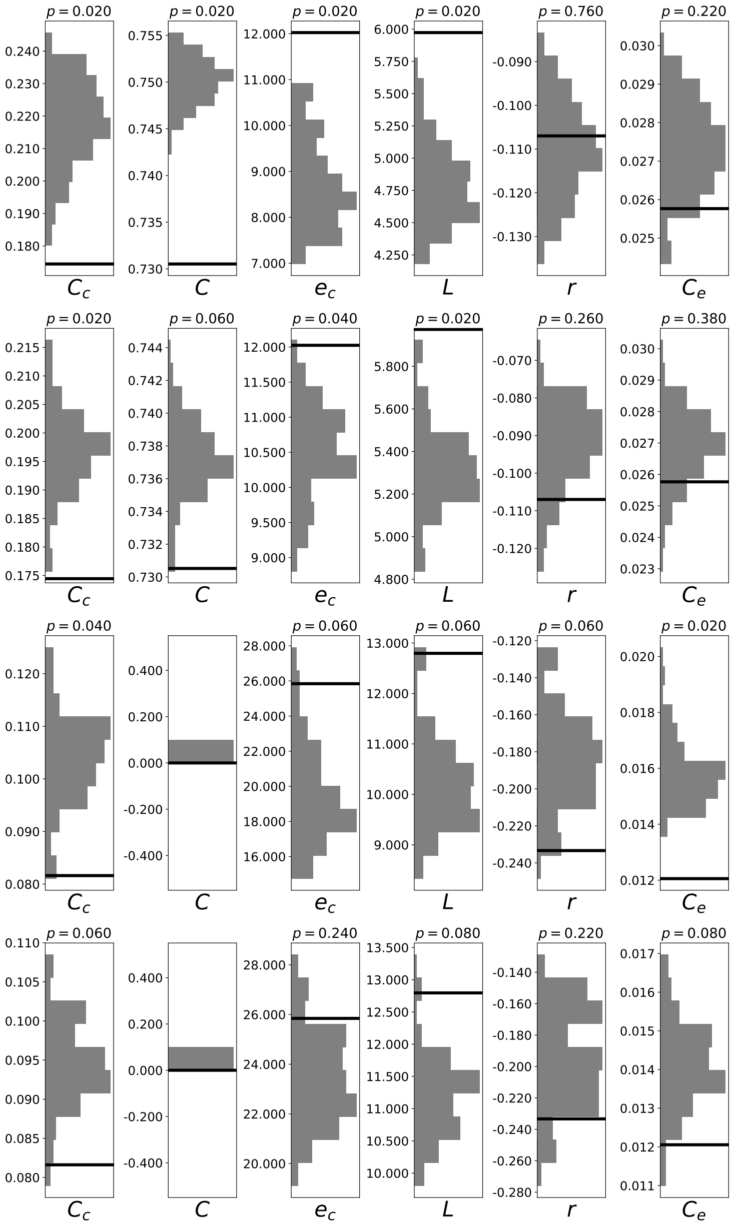


(a) Network from original data filtered using PMFG

(b) Network from marginally normalized data filtered using PMFG

(c) Network from original data filtered using MST

(d) Network from marginally normalized data filtered using MST

Figure 19: Global graph characteristics computed for unweighted networks constructed from real data (black bullets) and out of linearized surrogate datasets (gray bullets). Stocks considered were from SP500 index and there were 99 linear surrogates. Connectivity has been determined via mutual information for original and marginally normalized data. Presented characteristics are closeness $C_c$, average clustering coefficient $C$, eccentricity $e_C$, average shortest path $L$, assortative coefficient $r$ and eigenvalue centrality $C_e$. We use stocks traded between 11 November 2003 and 7 November 2013 and mutual information estimates have binning parameter equal to 4.

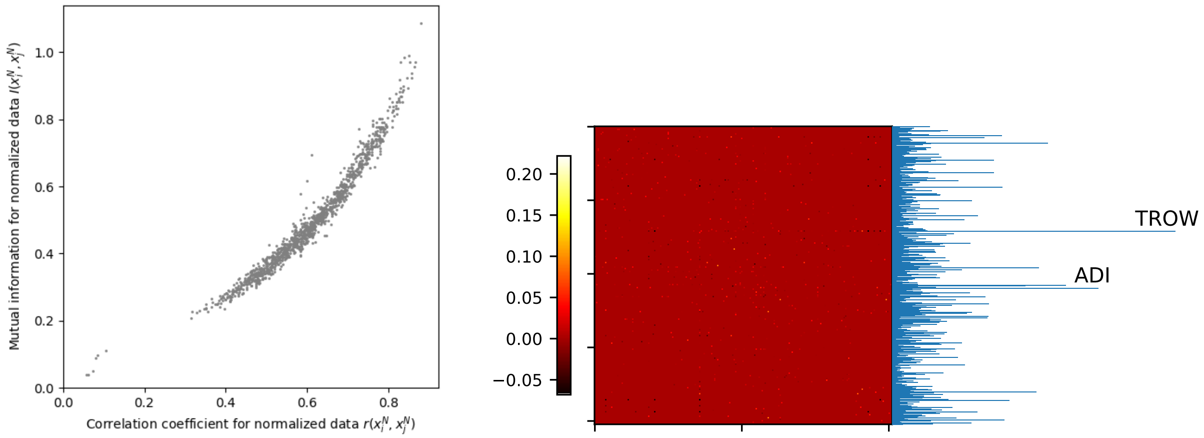


Figure 20: *Right*: Relation between correlation and mutual information estimates from the normalized filtered data data, i.e. only those later used for PMFG construction, having original setting similar as in Figure 2. *Left*: Extranormal information $I_e$ for normalized filtered data with summed rows and highlighted extremes.

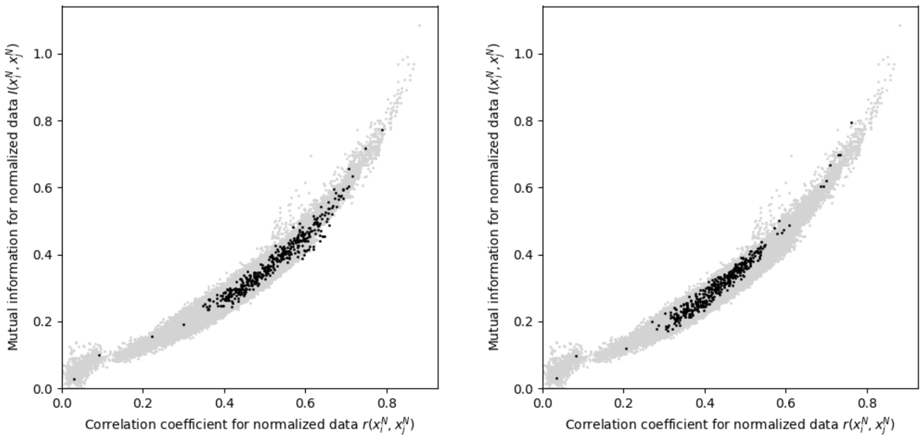


Figure 21: Relation between correlation and mutual information estimates computed from the normalized data having similar setting as in Figure 2 with one chosen highlighted stock in black. *Right*: the TROW stock . *Left*: the ADI stock.

Figure 23 contains results of nonlinearity analysis for networks using the WTA filtering.

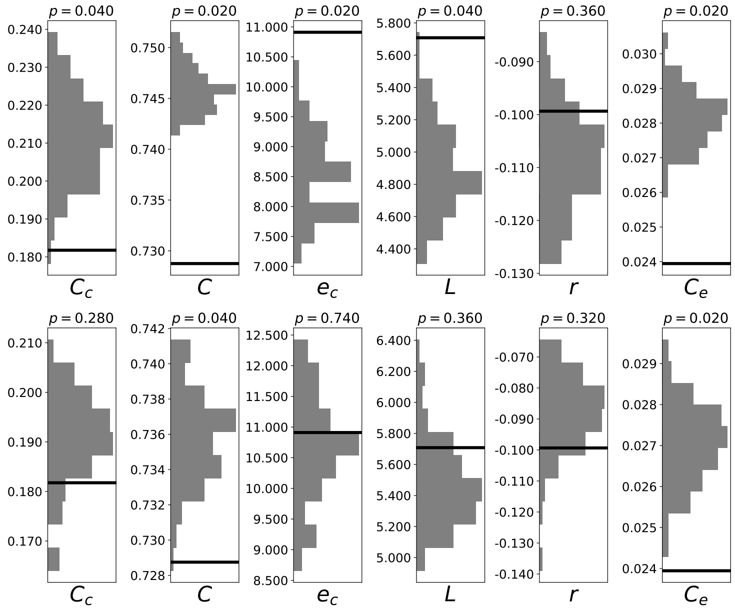


(a) Network from original data with stocks DD, TROW and ADI removed, filtered further using PMFG

(b) Network from marginally normalized data with stocks DD, TROW and ADI removed, filtered further using PMFG

Figure 22: Global graph characteristics computed for unweighted networks constructed out of real data (black bullets) and out of linearized surrogate datasets (gray bullets) both with stocks DD, TROW and ADI removed. Stocks considered were from SP500 index and there were 99 linear surrogates for which the same analysis has been computed. Connectivity has been determined via mutual information for original (above) and marginally normalized (below) data. Presented characteristics are closeness $C_c$, average clustering coefficient $C$, eccentricity $e_C$, average shortest path $L$, assortative coefficient $r$ and eigenvalue centrality $C_e$. We use stocks traded between 11 November 2003 and 7 November 2013 and mutual information estimates have binning parameter equal to 4.

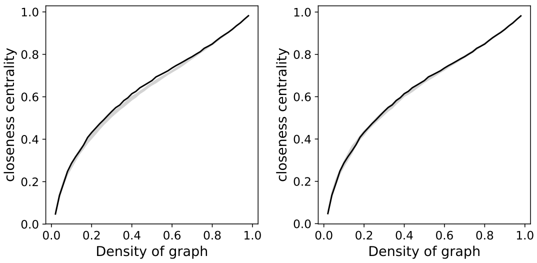


(a) Closeness centrality

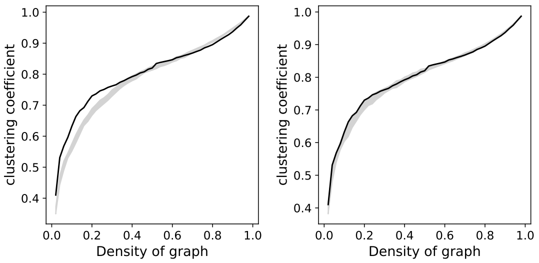


(b) Clustering coefficient

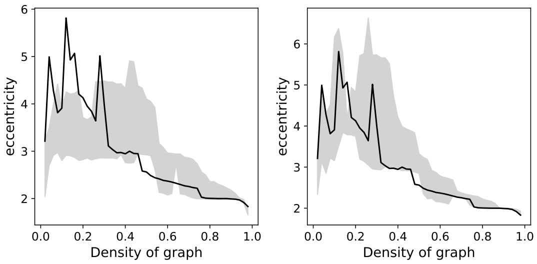


(c) Eccentricity

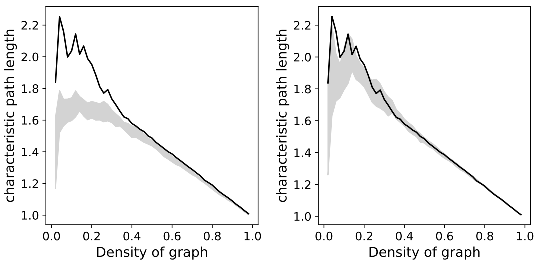


(d) Characteristic path length

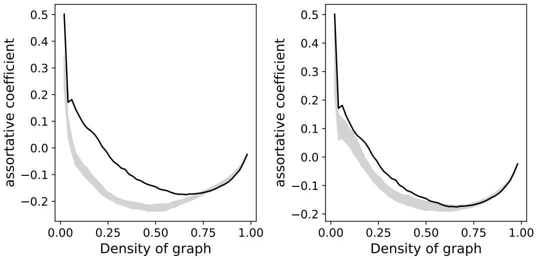


(e) Assortative coefficient

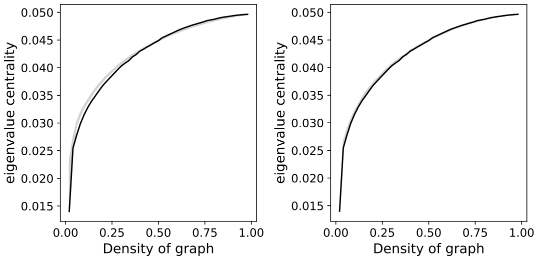


(f) Eigenvector centrality

Figure 23: Values of global graph characteristics each one plotted as function of density of network determined via winner-takes-all filtering across a range of densities from 0 to 0.98 with a step of 0.02. There were 99 linear surrogates for which the same analysis has been computed. Plots are data derived networks (black lines) and gray area representing interval of plots of linearized surrogate datasets (gray area). Considered network is constructed out of stocks from SP500 index with stock DD removed where connectivity has been determined via mutual information without any normalization (left) and with unvariatelly normalization applied (right). We use stocks traded between 11 November 2003 and 11 November 2008 and mutual information estimates have binning parameter equal to 4.
